# Supplementary material for: Electronic correlation in nearly free electron metals with beyond-DFT methods
Source: arXiv:2101.03262 source file (2022-07-29)
Supplement: Supplementary file 1 [file SupplementalMaterial.pdf]

# Supplemental Material: Electronic correlation in nearly free electron metals with beyond-DFT methods

Subhasish Mandal,[1] Kristjan Haule,[1] Karin M. Rabe,[1] and David Vanderbilt[1]
[1]*Department of Physics and Astronomy, Rutgers University, Piscataway, USA*

## CRYSTAL STRUCTURES

The experimental crystal structures are obtained from the ICSD-database. The ICSD numbers are given in Table I.

| Compound | ICSD-ID |
|---|---|
| Li | 44367 |
| Be | 1425 |
| Na | 196972 |
| Mg | 76748 |
| K | 44670 |
| Ca | 44348 |
| Rb | 44869 |
| Sr | 76162 |
| Cs | 42662 |
| Ba | 96587 |

TABLE I. ICSD-IDs for compounds studied here.

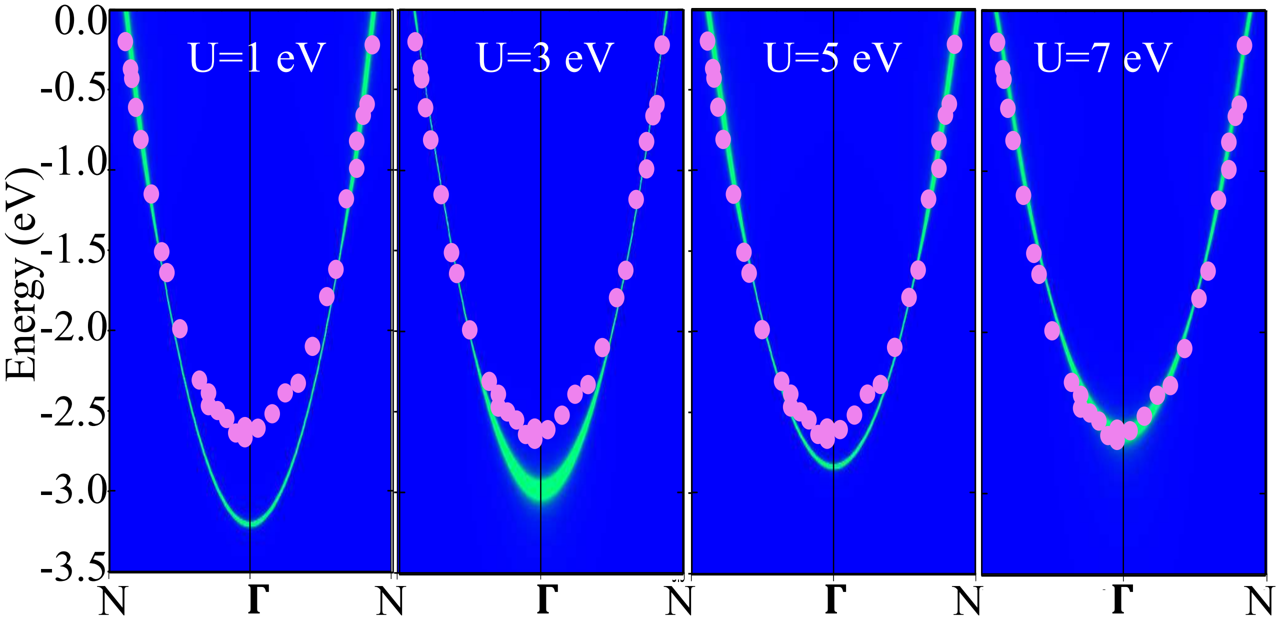


FIG. 1. (Color online) The dependence of Coulomb $U$ in eDMFT spectral function for elemental Na. Pink dots indicate angle-resolved-photoemission(ARPES) data from Ref. [11].

## RESULTS

In Figs. S2-S3, we describe band structures for elemental Be, Sr, Cs, Ca, and Rb as computed in LDA, mBJ, $G_0W_0$, B3LYP, and eDMFT in various energy windows.

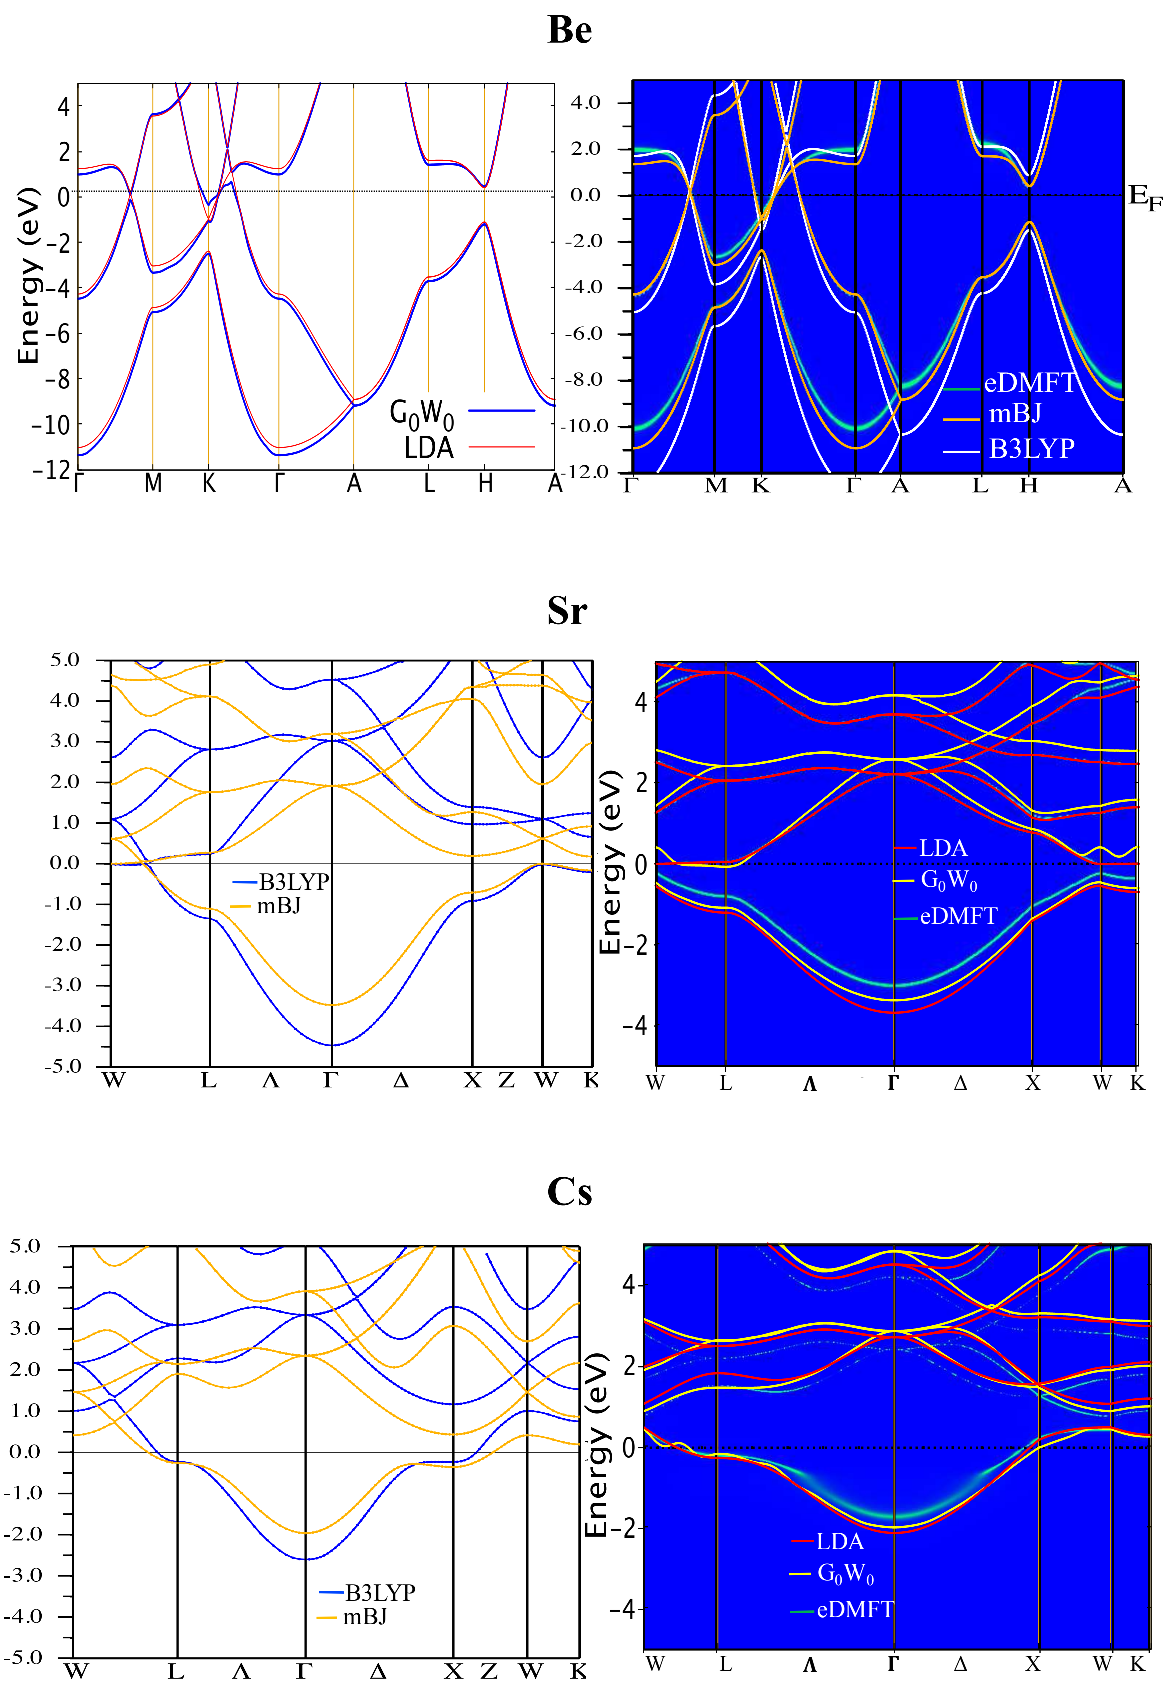


FIG. 2. (Color online) Band structures of elemental Be (top), Sr (middle) and Cs (bottom) as computed in LDA, mBJ, $G_0W_0$, B3LYP, and eDMFT.

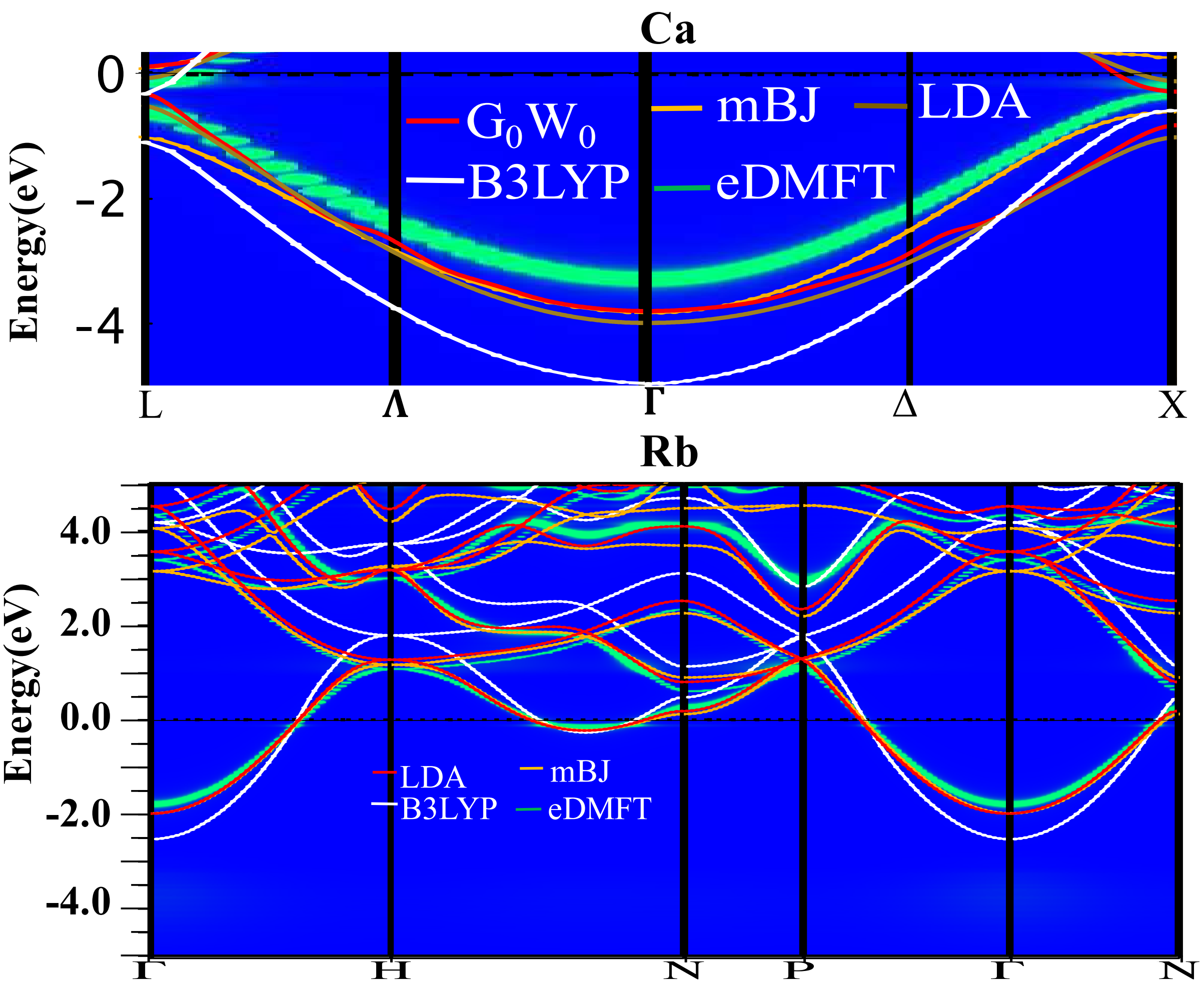


FIG. 3. (Color online) Band structures of elemental Ca (top) and Rb (bottom) as computed in LDA, mBJ, $G_0W_0$, B3LYP, and eDMFT.


[1] P. Blaha, K. Schwarz, G. Madsen, D. Kvasnicka, and J. Luitz, "An augmented plane wave plus local orbitals program for calculating crystal properties," (Vienna University of Technology, Austria, 2001, 2001).

[2] F. Tran and P. Blaha, Phys. Rev. Lett. **102**, 226401 (2009).

[3] A. D. Becke, The Journal of Chemical Physics **98**, 5648 (1993).

[4] F. Tran, P. Blaha, K. Schwarz, and P. Novák, Phys. Rev. B **74**, 155108 (2006).

[5] K. Haule and S. Mandal, arXiv:2008.07727 (2020).

[6] K. Haule, C.-H. Yee, and K. Kim, Phys. Rev. B **81**, 195107 (2010).

[7] K. Haule, Journal of the Physical Society of Japan **87**, 041005 (2018), https://doi.org/10.7566/JPSJ.87.041005.

[8] http:/hauleweb.rutgers.edu/tutorials.

[9] K. Haule, Physical Review B **75** (2007).

[10] K. Haule, Phys. Rev. Lett. **115**, 196403 (2015).

[11] I.-W. Lyo and E. W. Plummer, Phys. Rev. Lett. **60**, 1558 (1988).
